# Supplementary material for: Discrimination Between Quantum Common Causes and Quantum Causality
Source: arXiv:1806.10048 source file (2018-06-27)
Supplement: Supplementary file 1 [file SM1.pdf]

# The proof of Eq. (4) and Eq. (10)

## a. The proof of Eq. (4)

$\mathbf{P}(|\varphi\rangle)=\sum_{j=1}^{4} w_j{}^2 \bullet \mathbf{P}(|b_j\rangle)$ , where $|\varphi\rangle\in\mathbb{R}^4$ .

Proof. To prove $\mathbf{P}(|\varphi\rangle)=\sum_{j=1}^{4} w_j{}^2 \bullet \mathbf{P}(|b_j\rangle)$ , it is only necessary to prove $C_{ii}(|\varphi\rangle)=\sum_{j=1}^{4} w_j{}^2 \bullet C_{ii}(|b_j\rangle)(i=1,\cdots,3)$ . According to Eq. (1) and Eq. (3), $C_{ii}(|\varphi\rangle)=\sum_{j=1}^{4} w_j{}^2 \bullet C_{ii}(|b_j\rangle)$ is derived as follows.

$$
\begin{aligned}
&C_{11}(|\varphi\rangle)-\sum_{j=1}^{4} w_j{}^2 \bullet C_{11}(|b_j\rangle)\\
&=2p_{\varphi}(k=m\,|\,11)-1-\sum_{j=1}^{4} w_j{}^2\cdot[2p_{b_j}(k=m\,|\,11)-1]\\
&=2(\langle\varphi|\mathbf{P}_{x_0x_0}|\varphi\rangle+\langle\varphi|\mathbf{P}_{x_1x_1}|\varphi\rangle)-1-\sum_{j=1}^{4}\{w_j{}^2\cdot[2(\langle b_j|\mathbf{P}_{x_0x_0}|b_j\rangle+\langle b_j|\mathbf{P}_{x_1x_1}|b_j\rangle)-1]\}\\
&=2(\langle\varphi|\cdot(\mathbf{P}_{x_0x_0}+\mathbf{P}_{x_1x_1})\cdot|\varphi\rangle)-1-\sum_{j=1}^{4}\{w_j{}^2\cdot[2(\langle b_j|\cdot(\mathbf{P}_{x_0x_0}+\mathbf{P}_{x_1x_1})\cdot|b_j\rangle)-1]\}\\
&=2(\langle\varphi|\cdot(\mathbf{P}_{x_0x_0}+\mathbf{P}_{x_1x_1})\cdot|\varphi\rangle)-1-\sum_{j=1}^{4}\{w_j^2[2(\langle b_j|\cdot(\mathbf{P}_{x_0x_0}+\mathbf{P}_{x_1x_1})\cdot|b_j\rangle)-1]\}\\
&=2[\sum_{j=1}^{4}(w_j\cdot\langle b_j|)\cdot(\mathbf{P}_{x_0x_0}+\mathbf{P}_{x_1x_1})\cdot\sum_{j=1}^{4}(w_j\cdot|b_j\rangle)]-1-\sum_{j=1}^{4}\{w_j^2[2(\langle b_j|\cdot(\mathbf{P}_{x_0x_0}+\mathbf{P}_{x_1x_1})\cdot|b_j\rangle)-1]\}\\
&=0
\end{aligned}
$$

where $p_{\varphi}(k=m\,|\,11)$ ( $p_{b_j}(k=m\,|\,11)$ ) means that the probability of the same measurement results that the observable $\sigma_1\otimes\sigma_1$ is measured on two qubits $|\varphi\rangle$ (Bell state $|b_j\rangle$ $(j=1,\cdots,4)$ ). $\mathbf{P}_{x_0x_0}=|x_0x_0\rangle\langle x_0x_0|$, $\mathbf{P}_{x_1x_1}=|x_1x_1\rangle\langle x_1x_1|$, $\mathbf{P}_{x_0x_1}=|x_0x_1\rangle\langle x_0x_1|$, $\mathbf{P}_{x_1x_0}=|x_1x_0\rangle\langle x_1x_0|$ are a set of measurement operators.

Similarly, $C_{22}(|\varphi\rangle)=\sum_{j=1}^{4} w_j{}^2 \bullet C_{22}(|b_j\rangle)$ , $C_{33}(|\varphi\rangle)=\sum_{j=1}^{4} w_j{}^2 \bullet C_{33}(|b_j\rangle)$ .

## b. The proof of Eq. (10)

$\mathbf{P}(|\phi\rangle)=cos^2\alpha\cdot\mathbf{P}(|x\rangle)+sin^2\alpha\cdot\mathbf{P}(|y\rangle)$ , where $|\phi\rangle\in\mathbb{C}^4,|x\rangle,|y\rangle\in\mathbb{R}^4$

Proof. To prove $\mathbf{P}(|\phi\rangle)=cos^2\alpha\cdot\mathbf{P}(|x\rangle)+sin^2\alpha\cdot\mathbf{P}(|y\rangle)$ ,where $|\phi\rangle\in\mathbb{C}^4,|x\rangle,|y\rangle\in\mathbb{R}^4$ , it is only necessary to prove $C_{ii}(|\phi\rangle)=cos^2\alpha\cdot C_{ii}(|x\rangle)+sin^2\alpha\cdot C_{ii}(|y\rangle)(i=1,\cdots,3)$ . According to Eq. (1) and Eq. (9), Eq. (10) is derived as follows.

$$
\begin{aligned}
&C_{11}(|\phi\rangle)-cos^2\alpha\cdot C_{11}(|x\rangle)-sin^2\alpha\cdot C_{11}(|y\rangle)\\
&=2p_{\phi}(k=m\,|\,11)-1-cos^2\alpha\cdot[2p_x(k=m\,|\,11)-1]-sin^2\alpha\cdot[2p_y(k=m\,|\,11)-1]\\
&=2[p_{\phi}(k=m\,|\,11)-cos^2\alpha\cdot p_x(k=m\,|\,11)-sin^2\alpha\cdot p_y(k=m\,|\,11)]\\
&=2\{\langle\phi|\mathbf{P}_{x_0x_0}|\phi\rangle+\langle\phi|\mathbf{P}_{x_1x_1}|\phi\rangle)-cos^2\alpha\cdot[\langle x|\mathbf{P}_{x_0x_0}|x\rangle+\langle x|\mathbf{P}_{x_1x_1}|x\rangle)]-sin^2\alpha\cdot[\langle y|\mathbf{P}_{x_0x_0}|y\rangle+\langle y|\mathbf{P}_{x_1x_1}|y\rangle)]\}\\
&=2\{\langle\phi|\cdot(\mathbf{P}_{x_0x_0}+\mathbf{P}_{x_1x_1})\cdot|\phi\rangle-cos^2\alpha\cdot[\langle x|\cdot(\mathbf{P}_{x_0x_0}+\mathbf{P}_{x_1x_1})\cdot|x\rangle]-sin^2\alpha\cdot[\langle y|\cdot(\mathbf{P}_{x_0x_0}+\mathbf{P}_{x_1x_1})\cdot|y\rangle]\\
&=2[(cos\,\alpha\langle x|-isin\,\alpha\langle y|)\cdot(\mathbf{P}_{x_0x_0}+\mathbf{P}_{x_1x_1})\cdot(cos\,\alpha|x\rangle+isin\,\alpha|y\rangle)-cos^2\alpha[\langle x|(\mathbf{P}_{x_0x_0}+\mathbf{P}_{x_1x_1})|x\rangle]-sin^2\alpha[\langle y|(\mathbf{P}_{x_0x_0}+\mathbf{P}_{x_1x_1})|y\rangle]\\
&=0
\end{aligned}
$$

where $p_{\phi}(k=m\,|\,11)$ ( $p_x(k=m\,|\,11),p_y(k=m\,|\,11)$ ) means that the probability of the same measurement results that the observable $\sigma_1\otimes\sigma_1$ is measured on two qubits $|\phi\rangle$ ( $|x\rangle,|y\rangle$ ).

Similarly, $C_{22}(|\phi\rangle)=cos^2\alpha\cdot C_{22}(|x\rangle)-sin^2\alpha\cdot C_{22}(|y\rangle)$ , $C_{33}(|\phi\rangle)=cos^2\alpha\cdot C_{33}(|x\rangle)-sin^2\alpha\cdot C_{33}(|y\rangle)$ .

# All extreme points of $C_{CC}$

| i | $\langle\varphi|$ | λ | i | $\langle\varphi|$ | λ |
|---|---|---|---|---|---|
| 1 | ( -0.707107 , -0.707107 , 0.000000 , 0.000000) | 0.000000 | 68 | ( -0.816497 , -0.408248 , 0.408248 , 0.000000) | 0.000000 |
| 2 | ( 0.707107 , -0.707107 , 0.000000 , 0.000000) | 0.000000 | 69 | ( 0.816497 , -0.408248 , 0.408248 , 0.000000) | 0.000000 |
| 3 | ( -0.707107 , 0.707107 , 0.000000 , 0.000000) | 0.000000 | 70 | ( -0.408248 , -0.816497 , 0.000000 , -0.408248) | 0.000000 |
| 4 | ( 0.707107 , 0.707107 , 0.000000 , 0.000000) | 0.000000 | 71 | ( 0.408248 , -0.816497 , 0.000000 , -0.408248) | 0.000000 |
| 5 | ( -0.707107 , 0.000000 , -0.707107 , 0.000000) | 0.000000 | 72 | ( -0.408248 , 0.816497 , 0.000000 , -0.408248) | 0.000000 |
| 6 | ( 0.707107 , 0.000000 , -0.707107 , 0.000000) | 0.000000 | 73 | ( 0.408248 , 0.816497 , 0.000000 , -0.408248) | 0.000000 |
| 7 | ( -0.707107 , 0.000000 , 0.707107 , 0.000000) | 0.000000 | 74 | ( -0.408248 , -0.816497 , 0.000000 , 0.408248) | 0.000000 |
| 8 | ( 0.707107 , 0.000000 , 0.707107 , 0.000000) | 0.000000 | 75 | ( 0.408248 , -0.816497 , 0.000000 , 0.408248) | 0.000000 |
| 9 | ( 1.000000 , 0.000000 , 0.000000 , 0.000000) | 0.000000 | 76 | ( -0.408248 , 0.816497 , 0.000000 , 0.408248) | 0.000000 |
| 10 | ( 0.000000 , 1.000000 , 0.000000 , 0.000000) | 0.000000 | 77 | ( 0.408248 , 0.816497 , 0.000000 , 0.408248) | 0.000000 |
| 11 | ( 0.000000 , 0.000000 , 1.000000 , 0.000000) | 0.000000 | 78 | ( -0.408248 , 0.000000 , -0.816497 , -0.408248) | 0.000000 |
| 12 | ( -0.577350 , -0.408248 , -0.577350 , -0.408248) | 0.000000 | 79 | ( 0.408248 , 0.000000 , -0.816497 , -0.408248) | 0.000000 |
| 13 | ( 0.577350 , -0.408248 , -0.577350 , -0.408248) | 0.000000 | 80 | ( -0.408248 , 0.000000 , 0.816497 , -0.408248) | 0.000000 |
| 14 | ( -0.577350 , 0.408248 , -0.577350 , -0.408248) | 0.000000 | 81 | ( 0.408248 , 0.000000 , 0.816497 , -0.408248) | 0.000000 |
| 15 | ( 0.577350 , 0.408248 , -0.577350 , -0.408248) | 0.000000 | 82 | ( -0.408248 , 0.000000 , -0.816497 , 0.408248) | 0.000000 |
| 16 | ( -0.577350 , -0.408248 , 0.577350 , -0.408248) | 0.000000 | 83 | ( 0.408248 , 0.000000 , -0.816497 , 0.408248) | 0.000000 |
| 17 | ( 0.577350 , -0.408248 , 0.577350 , -0.408248) | 0.000000 | 84 | ( -0.408248 , 0.000000 , 0.816497 , 0.408248) | 0.000000 |
| 18 | ( -0.577350 , 0.408248 , 0.577350 , -0.408248) | 0.000000 | 85 | ( 0.408248 , 0.000000 , 0.816497 , 0.408248) | 0.000000 |
| 19 | ( 0.577350 , 0.408248 , 0.577350 , -0.408248) | 0.000000 | 86 | ( 0.000000 , 0.408248 , -0.408248 , -0.816497) | 0.000000 |
| 20 | ( -0.577350 , -0.577350 , -0.408248 , -0.408248) | 0.000000 | 87 | ( 0.000000 , -0.408248 , 0.408248 , -0.816497) | 0.000000 |
| 21 | ( 0.577350 , -0.577350 , -0.408248 , -0.408248) | 0.000000 | 88 | ( 0.000000 , 0.408248 , -0.408248 , 0.816497) | 0.000000 |
| 22 | ( -0.577350 , 0.577350 , -0.408248 , -0.408248) | 0.000000 | 89 | ( 0.000000 , -0.408248 , 0.408248 , 0.816497) | 0.000000 |
| 23 | ( 0.577350 , 0.577350 , -0.408248 , -0.408248) | 0.000000 | 90 | ( -0.816497 , -0.408248 , -0.408248 , 0.000000) | 0.444444 |
| 24 | ( -0.577350 , -0.577350 , 0.408248 , -0.408248) | 0.000000 | 91 | ( 0.816497 , -0.408248 , -0.408248 , 0.000000) | 0.444444 |
| 25 | ( 0.577350 , -0.577350 , 0.408248 , -0.408248) | 0.000000 | 92 | ( -0.816497 , 0.408248 , 0.408248 , 0.000000) | 0.444444 |
| 26 | ( -0.577350 , 0.577350 , 0.408248 , -0.408248) | 0.000000 | 93 | ( 0.816497 , 0.408248 , 0.408248 , 0.000000) | 0.444444 |
| 27 | ( 0.577350 , 0.577350 , 0.408248 , -0.408248) | 0.000000 | 94 | ( 0.000000 , -0.408248 , -0.408248 , -0.816497) | 0.444444 |
| 28 | ( -0.577350 , -0.408248 , -0.577350 , 0.408248) | 0.000000 | 95 | ( 0.000000 , 0.408248 , 0.408248 , -0.816497) | 0.444444 |
| 29 | ( 0.577350 , -0.408248 , -0.577350 , 0.408248) | 0.000000 | 96 | ( 0.000000 , -0.408248 , -0.408248 , 0.816497) | 0.444444 |
| 30 | ( -0.577350 , 0.408248 , -0.577350 , 0.408248) | 0.000000 | 97 | ( 0.000000 , 0.408248 , 0.408248 , 0.816497) | 0.444444 |
| 31 | ( 0.577350 , 0.408248 , -0.577350 , 0.408248) | 0.000000 | 98 | ( -1.000000 , 0.000000 , 0.000000 , 0.000000) | 0.000000 |
| 32 | ( -0.577350 , -0.408248 , 0.577350 , 0.408248) | 0.000000 | 99 | ( -0.707107 , -0.707107 , 0.000000 , 0.000000) | 0.000000 |
| 33 | ( 0.577350 , -0.408248 , 0.577350 , 0.408248) | 0.000000 | 100 | ( 0.707107 , -0.707107 , 0.000000 , 0.000000) | 0.000000 |
| 34 | ( -0.577350 , 0.408248 , 0.577350 , 0.408248) | 0.000000 | 101 | ( -0.707107 , 0.707107 , 0.000000 , 0.000000) | 0.000000 |
| 35 | ( 0.577350 , 0.408248 , 0.577350 , 0.408248) | 0.000000 | 102 | ( 0.707107 , 0.707107 , 0.000000 , 0.000000) | 0.000000 |
| 36 | ( -0.577350 , -0.577350 , -0.408248 , 0.408248) | 0.000000 | 103 | ( -0.707107 , 0.000000 , -0.707107 , 0.000000) | 0.000000 |
| 37 | ( 0.577350 , -0.577350 , -0.408248 , 0.408248) | 0.000000 | 104 | ( 0.707107 , 0.000000 , -0.707107 , 0.000000) | 0.000000 |
| 38 | ( -0.577350 , 0.577350 , -0.408248 , 0.408248) | 0.000000 | 105 | ( -0.707107 , 0.000000 , 0.707107 , 0.000000) | 0.000000 |
| 39 | ( 0.577350 , 0.577350 , -0.408248 , 0.408248) | 0.000000 | 106 | ( 0.707107 , 0.000000 , 0.707107 , 0.000000) | 0.000000 |
| 40 | ( -0.577350 , -0.577350 , 0.408248 , 0.408248) | 0.000000 | 107 | ( 0.000000 , 0.707107 , -0.707107 , 0.000000) | 0.000000 |
| 41 | ( 0.577350 , -0.577350 , 0.408248 , 0.408248) | 0.000000 | 108 | ( 0.000000 , -0.707107 , 0.707107 , 0.000000) | 0.000000 |
| 42 | ( -0.577350 , 0.577350 , 0.408248 , 0.408248) | 0.000000 | 109 | ( 0.000000 , -0.707107 , 0.000000 , -0.707107) | 0.000000 |
| 43 | ( 0.577350 , 0.577350 , 0.408248 , 0.408248) | 0.000000 | 110 | ( 0.000000 , 0.707107 , 0.000000 , -0.707107) | 0.000000 |
| 44 | ( 0.000000 , -1.000000 , 0.000000 , 0.000000) | 0.000000 | 111 | ( 0.000000 , -0.707107 , 0.000000 , 0.707107) | 0.000000 |
| 45 | ( 0.000000 , 1.000000 , 0.000000 , 0.000000) | 0.000000 | 112 | ( 0.000000 , 0.707107 , 0.000000 , 0.707107) | 0.000000 |
| 46 | ( 0.000000 , 0.000000 , -1.000000 , 0.000000) | 0.000000 | 113 | ( 0.000000 , 0.000000 , -0.707107 , -0.707107) | 0.000000 |
| 47 | ( 0.000000 , 0.000000 , 1.000000 , 0.000000) | 0.000000 | 114 | ( 0.000000 , 0.000000 , 0.707107 , -0.707107) | 0.000000 |
| 48 | ( 0.000000 , 0.000000 , 0.000000 , -1.000000) | 0.000000 | 115 | ( 0.000000 , 0.000000 , -0.707107 , 0.707107) | 0.000000 |
| 49 | ( 0.000000 , 0.000000 , 0.000000 , 1.000000) | 0.000000 | 116 | ( 0.000000 , 0.000000 , 0.707107 , 0.707107) | 0.000000 |
| 50 | ( -0.500000 , -0.500000 , -0.500000 , -0.500000) | 0.000000 | 117 | ( 0.000000 , -0.577350 , 0.000000 , -0.816497) | 0.000000 |
| 51 | ( 0.500000 , -0.500000 , -0.500000 , -0.500000) | 0.000000 | 118 | ( 0.000000 , 0.577350 , 0.000000 , -0.816497) | 0.000000 |
| 52 | ( -0.500000 , 0.500000 , -0.500000 , -0.500000) | 0.000000 | 119 | ( 0.000000 , -0.577350 , 0.000000 , 0.816497) | 0.000000 |
| 53 | ( 0.500000 , 0.500000 , -0.500000 , -0.500000) | 0.000000 | 120 | ( 0.000000 , 0.577350 , 0.000000 , 0.816497) | 0.000000 |
| 54 | ( -0.500000 , -0.500000 , 0.500000 , -0.500000) | 0.000000 | 121 | ( 0.000000 , 0.000000 , -0.577350 , -0.816497) | 0.000000 |
| 55 | ( 0.500000 , -0.500000 , 0.500000 , -0.500000) | 0.000000 | 122 | ( 0.000000 , 0.000000 , 0.577350 , -0.816497) | 0.000000 |
| 56 | ( -0.500000 , 0.500000 , 0.500000 , -0.500000) | 0.000000 | 123 | ( 0.000000 , 0.000000 , -0.577350 , 0.816497) | 0.000000 |
| 57 | ( 0.500000 , 0.500000 , 0.500000 , -0.500000) | 0.000000 | 124 | ( 0.000000 , 0.000000 , 0.577350 , 0.816497) | 0.000000 |
| 58 | ( -0.500000 , -0.500000 , -0.500000 , 0.500000) | 0.000000 | 125 | ( 0.000000 , -0.707107 , -0.707107 , 0.000000) | -4.000000 |
| 59 | ( 0.500000 , -0.500000 , -0.500000 , 0.500000) | 0.000000 | 126 | ( 0.000000 , 0.707107 , 0.707107 , 0.000000) | -4.000000 |
| 60 | ( -0.500000 , 0.500000 , -0.500000 , 0.500000) | 0.000000 | 127 | ( -0.707107 , 0.000000 , 0.000000 , -0.707107) | -4.000000 |
| 61 | ( 0.500000 , 0.500000 , -0.500000 , 0.500000) | 0.000000 | 128 | ( 0.707107 , 0.000000 , 0.000000 , -0.707107) | -4.000000 |
| 62 | ( -0.500000 , -0.500000 , 0.500000 , 0.500000) | 0.000000 | 129 | ( -0.707107 , 0.000000 , 0.000000 , 0.707107) | -4.000000 |
| 63 | ( 0.500000 , -0.500000 , 0.500000 , 0.500000) | 0.000000 | 130 | ( 0.707107 , 0.000000 , 0.000000 , 0.707107) | -4.000000 |
| 64 | ( -0.500000 , 0.500000 , 0.500000 , 0.500000) | 0.000000 | 131 | ( -0.912871 , 0.000000 , -0.408248 , 0.000000) | 0.000000 |
| 65 | ( 0.500000 , 0.500000 , 0.500000 , 0.500000) | 0.000000 | 132 | ( 0.912871 , 0.000000 , -0.408248 , 0.000000) | 0.000000 |
| 66 | ( -0.816497 , 0.408248 , -0.408248 , 0.000000) | 0.000000 | 133 | ( -0.912871 , 0.000000 , 0.408248 , 0.000000) | 0.000000 |
| 67 | ( 0.816497 , 0.408248 , -0.408248 , 0.000000) | 0.000000 | 134 | ( 0.912871 , 0.000000 , 0.408248 , 0.000000) | 0.000000 |

Table I. All extreme points of $C_{CC}$. i stands for the ith extreme point, $\langle\varphi|$ is the conjugate transposed vector of the quantum state $|\varphi\rangle$, λ is a Lagrangian multiplier, the detail see Eq. (7) .

# All extreme points of $C_{\mathrm{DC}}$

| i | $\sqrt{p_0}$ | $\sqrt{p_1}$ | $\sqrt{p_2}$ | $\sqrt{p_3}$ | λ | i | $\sqrt{p_0}$ | $\sqrt{p_1}$ | $\sqrt{p_2}$ | $\sqrt{p_3}$ | λ |
|---|---|---|---|---|---|---|---|---|---|---|---|
| 1 | -0.707107 | -0.707107 | 0.000000 | 0.000000 | 0.000000 | 47 | -0.577350 | 0.577350 | 0.000000 | -0.577350 | -0.111111 |
| 2 | 0.707107 | -0.707107 | 0.000000 | 0.000000 | 0.000000 | 48 | 0.577350 | 0.577350 | 0.000000 | -0.577350 | -0.111111 |
| 3 | -0.707107 | 0.707107 | 0.000000 | 0.000000 | 0.000000 | 49 | -0.577350 | -0.577350 | 0.000000 | 0.577350 | -0.111111 |
| 4 | 0.707107 | 0.707107 | 0.000000 | 0.000000 | 0.000000 | 50 | 0.577350 | -0.577350 | 0.000000 | 0.577350 | -0.111111 |
| 5 | -0.707107 | 0.000000 | -0.707107 | 0.000000 | 0.000000 | 51 | -0.577350 | 0.577350 | 0.000000 | 0.577350 | -0.111111 |
| 6 | 0.707107 | 0.000000 | -0.707107 | 0.000000 | 0.000000 | 52 | 0.577350 | 0.577350 | 0.000000 | 0.577350 | -0.111111 |
| 7 | 0.000000 | -0.707107 | -0.707107 | 0.000000 | 0.000000 | 53 | -0.577350 | 0.000000 | -0.577350 | -0.577350 | -0.111111 |
| 8 | 0.000000 | 0.707107 | -0.707107 | 0.000000 | 0.000000 | 54 | 0.577350 | 0.000000 | -0.577350 | -0.577350 | -0.111111 |
| 9 | -0.707107 | 0.000000 | 0.707107 | 0.000000 | 0.000000 | 55 | -0.577350 | 0.000000 | 0.577350 | -0.577350 | -0.111111 |
| 10 | 0.707107 | 0.000000 | 0.707107 | 0.000000 | 0.000000 | 56 | 0.577350 | 0.000000 | 0.577350 | -0.577350 | -0.111111 |
| 11 | 0.000000 | -0.707107 | 0.707107 | 0.000000 | 0.000000 | 57 | -0.577350 | 0.000000 | -0.577350 | 0.577350 | -0.111111 |
| 12 | 0.000000 | 0.707107 | 0.707107 | 0.000000 | 0.000000 | 58 | 0.577350 | 0.000000 | -0.577350 | 0.577350 | -0.111111 |
| 13 | -1.000000 | 0.000000 | 0.000000 | 0.000000 | 3.000000 | 59 | -0.577350 | 0.000000 | 0.577350 | 0.577350 | -0.111111 |
| 14 | 1.000000 | 0.000000 | 0.000000 | 0.000000 | 3.000000 | 60 | 0.577350 | 0.000000 | 0.577350 | 0.577350 | -0.111111 |
| 15 | 0.000000 | -1.000000 | 0.000000 | 0.000000 | 3.000000 | 61 | 0.000000 | -0.577350 | -0.577350 | -0.577350 | -0.111111 |
| 16 | 0.000000 | 1.000000 | 0.000000 | 0.000000 | 3.000000 | 62 | 0.000000 | 0.577350 | -0.577350 | -0.577350 | -0.111111 |
| 17 | 0.000000 | 0.000000 | -1.000000 | 0.000000 | 3.000000 | 63 | 0.000000 | -0.577350 | 0.577350 | -0.57730 | -0.111111 |
| 18 | 0.000000 | 0.000000 | 1.000000 | 0.000000 | 3.000000 | 64 | 0.000000 | 0.577350 | 0.577350 | -0.57735 | -0.111111 |
| 19 | 0.000000 | 0.000000 | 0.000000 | -1.000000 | 3.000000 | 65 | 0.000000 | -0.577350 | -0.577350 | 0.577350 | -0.111111 |
| 20 | 0.000000 | 0.000000 | 0.000000 | 1.000000 | 3.000000 | 66 | 0.000000 | 0.577350 | -0.577350 | 0.577350 | -0.111111 |
| 21 | -0.500000 | -0.500000 | -0.500000 | -0.500000 | 0.000000 | 67 | 0.000000 | -0.577350 | 0.577350 | 0.577350 | -0.111111 |
| 22 | 0.500000 | -0.500000 | -0.500000 | -0.500000 | 0.000000 | 68 | 0.000000 | 0.577350 | 0.577350 | 0.577350 | -0.111111 |
| 23 | -0.500000 | 0.500000 | -0.500000 | -0.500000 | 0.000000 | 69 | -0.707107 | -0.707107 | 0.000000 | 0.000000 | 0.000000 |
| 24 | 0.500000 | 0.500000 | -0.500000 | -0.500000 | 0.000000 | 70 | 0.707107 | -0.707107 | 0.000000 | 0.000000 | 0.000000 |
| 25 | -0.500000 | -0.500000 | 0.500000 | -0.500000 | 0.000000 | 71 | -0.707107 | 0.707107 | 0.000000 | 0.000000 | 0.000000 |
| 26 | 0.500000 | -0.500000 | 0.500000 | -0.500000 | 0.000000 | 72 | 0.707107 | 0.707107 | 0.000000 | 0.000000 | 0.000000 |
| 27 | -0.500000 | 0.500000 | 0.500000 | -0.500000 | 0.000000 | 73 | -0.707107 | 0.000000 | -0.707107 | 0.000000 | 0.000000 |
| 28 | 0.500000 | 0.500000 | 0.500000 | -0.500000 | 0.000000 | 74 | 0.707107 | 0.000000 | -0.707107 | 0.000000 | 0.000000 |
| 29 | -0.500000 | -0.500000 | -0.500000 | 0.500000 | 0.000000 | 75 | -0.707107 | 0.000000 | 0.707107 | 0.000000 | 0.000000 |
| 30 | 0.500000 | -0.500000 | -0.500000 | 0.500000 | 0.000000 | 76 | 0.707107 | 0.000000 | 0.707107 | 0.000000 | 0.000000 |
| 31 | -0.500000 | 0.500000 | -0.500000 | 0.500000 | 0.000000 | 77 | 0.000000 | -0.707107 | -0.707107 | 0.000000 | 0.000000 |
| 32 | 0.500000 | 0.500000 | -0.500000 | 0.500000 | 0.000000 | 78 | 0.000000 | 0.707107 | -0.707107 | 0.000000 | 0.000000 |
| 33 | -0.500000 | -0.500000 | 0.500000 | 0.500000 | 0.000000 | 79 | 0.000000 | -0.707107 | 0.707107 | 0.000000 | 0.000000 |
| 34 | 0.500000 | -0.500000 | 0.500000 | 0.500000 | 0.000000 | 80 | 0.000000 | 0.707107 | 0.707107 | 0.000000 | 0.000000 |
| 35 | -0.500000 | 0.500000 | 0.500000 | 0.500000 | 0.000000 | 81 | -0.707107 | 0.000000 | 0.000000 | -0.707107 | 0.000000 |
| 36 | 0.500000 | 0.500000 | 0.500000 | 0.500000 | 0.000000 | 82 | 0.707107 | 0.000000 | 0.000000 | -0.707107 | 0.000000 |
| 37 | -0.577350 | -0.577350 | -0.577350 | 0.000000 | -0.111111 | 83 | -0.707107 | 0.000000 | 0.000000 | 0.707107 | 0.000000 |
| 38 | 0.577350 | -0.577350 | -0.577350 | 0.000000 | -0.111111 | 84 | 0.707107 | 0.000000 | 0.000000 | 0.707107 | 0.000000 |
| 39 | -0.577350 | 0.577350 | -0.577350 | 0.000000 | -0.111111 | 85 | 0.000000 | -0.707107 | 0.000000 | -0.707107 | 0.000000 |
| 40 | 0.577350 | 0.577350 | -0.577350 | 0.000000 | -0.111111 | 86 | 0.000000 | 0.707107 | 0.000000 | -0.707107 | 0.000000 |
| 41 | -0.577350 | -0.577350 | 0.577350 | 0.000000 | -0.111111 | 87 | 0.000000 | -0.707107 | 0.000000 | 0.707107 | 0.000000 |
| 42 | 0.577350 | -0.577350 | 0.577350 | 0.000000 | -0.111111 | 88 | 0.000000 | 0.707107 | 0.000000 | 0.707107 | 0.000000 |
| 43 | -0.577350 | 0.577350 | 0.577350 | 0.000000 | -0.111111 | 89 | 0.000000 | 0.000000 | -0.707107 | -0.707107 | 0.000000 |
| 44 | 0.577350 | 0.577350 | 0.577350 | 0.000000 | -0.111111 | 90 | 0.000000 | 0.000000 | 0.707107 | -0.707107 | 0.000000 |
| 45 | -0.577350 | -0.577350 | 0.000000 | -0.577350 | -0.111111 | 91 | 0.000000 | 0.000000 | -0.707107 | 0.707107 | 0.000000 |
| 46 | 0.577350 | -0.577350 | 0.000000 | -0.577350 | -0.111111 | 92 | 0.000000 | 0.000000 | 0.707107 | 0.707107 | 0.000000 |

Table II. All extreme points of $C_{\mathrm{DC}}$. i stands for the ith extreme point, $p_i (j = 0, \cdots, 3)$ is convex combination coefficients and λ is a Lagrangian multiplier, the detail see Eq. (24).
